# Supplementary material for: Evaluating Adversarial Robustness in the Spatial Frequency Domain
Source: arXiv:2405.06345 source file (2024-05-10)
Supplement: Supplementary file 1 [file gradcam_simple.tex]

\captionsetup[subfigure]{labelformat=empty}
\begin{figure*}[t]
    \centering
    % Golf
    \begin{subfigure}{.075\linewidth}
        \centering
        \includegraphics[width=.98\linewidth]{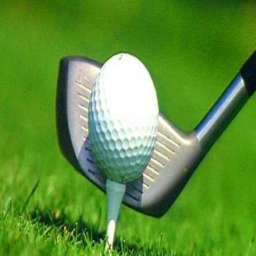}
        \includegraphics[width=.98\linewidth]{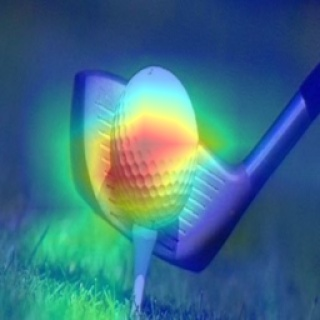}
        \includegraphics[width=.98\linewidth]{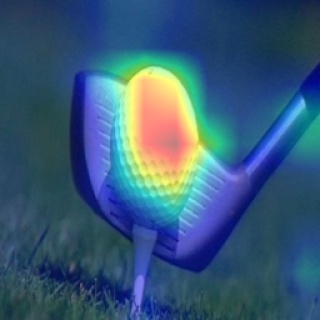}
        \caption{$\epsilon = 0$}
    \end{subfigure}
    \begin{subfigure}{.075\linewidth}
        \centering
        \includegraphics[width=.98\linewidth]{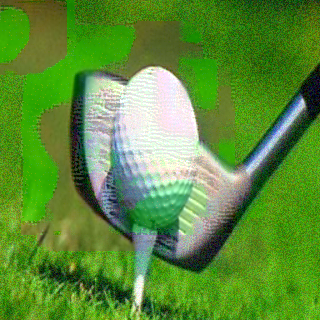}
        \includegraphics[width=.98\linewidth]{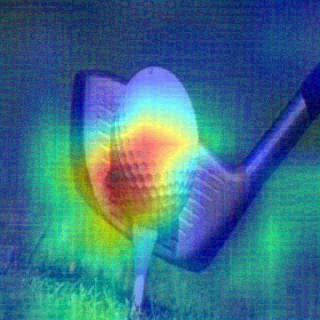}
        \includegraphics[width=.98\linewidth]{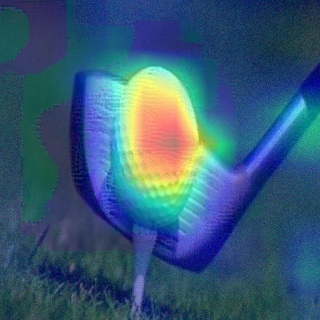}
        \caption{$\epsilon = 0.1$}
    \end{subfigure}
    \begin{subfigure}{.075\linewidth}
        \centering
        \includegraphics[width=.98\linewidth]{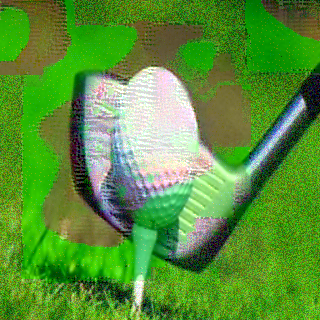}
        \includegraphics[width=.98\linewidth]{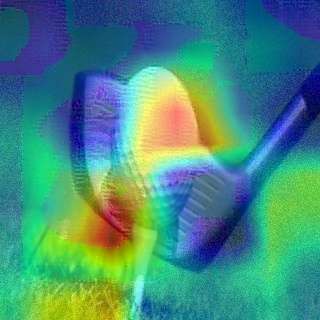}
        \includegraphics[width=.98\linewidth]{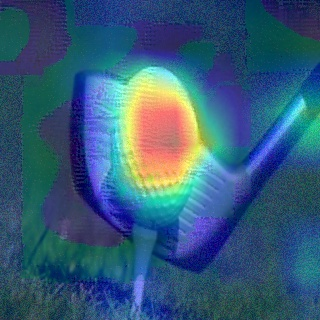}
        \caption{$\epsilon = 0.2$}
    \end{subfigure}
    \begin{subfigure}{.075\linewidth}
        \centering
        \includegraphics[width=.98\linewidth]{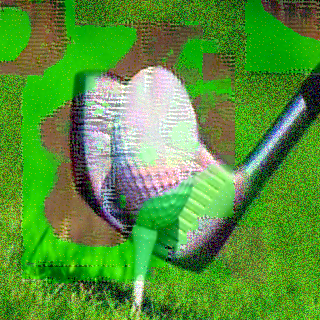}
        \includegraphics[width=.98\linewidth]{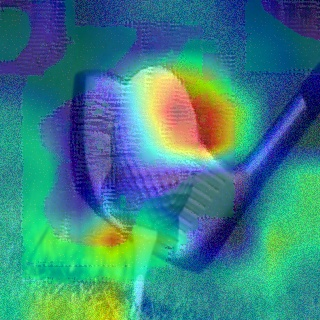}
        \includegraphics[width=.98\linewidth]{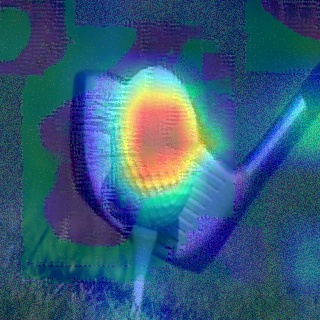}
        \caption{$\epsilon = 0.3$}
    \end{subfigure}
    % gas
    \centering
    \begin{subfigure}{.075\linewidth}
        \centering
        \includegraphics[width=.98\linewidth]{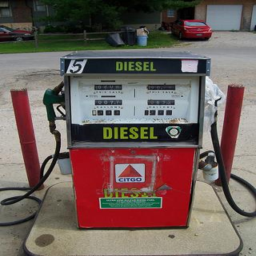}
        \includegraphics[width=.98\linewidth]{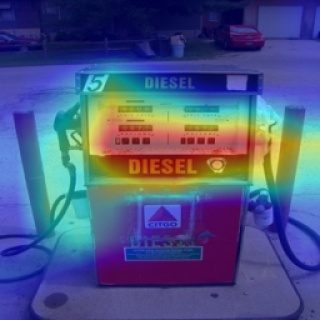}
        \includegraphics[width=.98\linewidth]{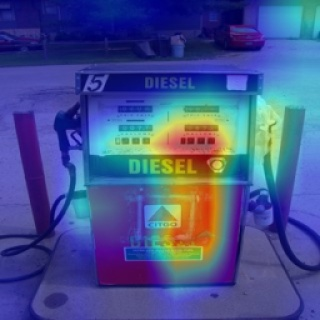}
        \caption{$\epsilon = 0$}
    \end{subfigure}
    \begin{subfigure}{.075\linewidth}
        \centering
        \includegraphics[width=.98\linewidth]{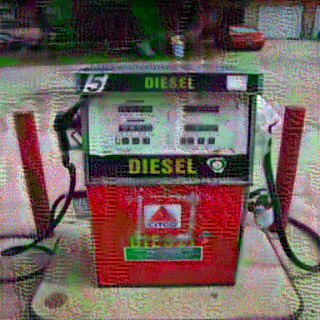}
        \includegraphics[width=.98\linewidth]{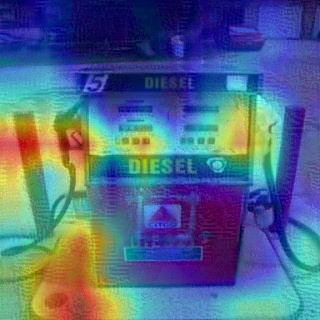}
        \includegraphics[width=.98\linewidth]{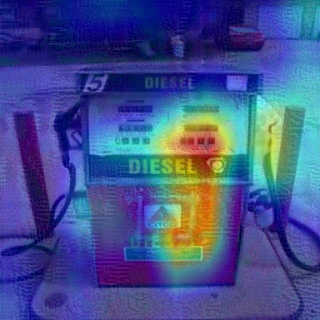}
        \caption{$\epsilon = 0.1$}
    \end{subfigure}
    \begin{subfigure}{.075\linewidth}
        \centering
        \includegraphics[width=.98\linewidth]{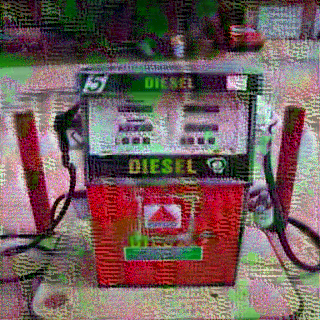}
        \includegraphics[width=.98\linewidth]{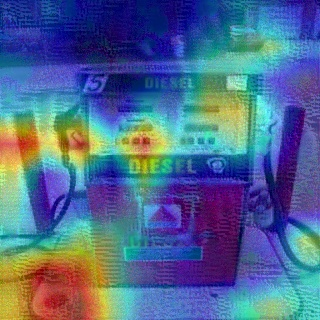}
        \includegraphics[width=.98\linewidth]{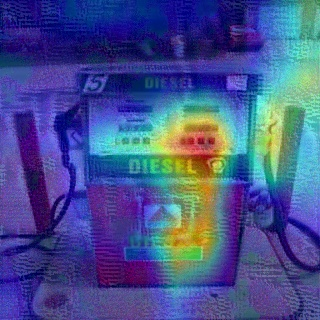}
        \caption{$\epsilon = 0.2$}
    \end{subfigure}
    \begin{subfigure}{.075\linewidth}
        \centering
        \includegraphics[width=.98\linewidth]{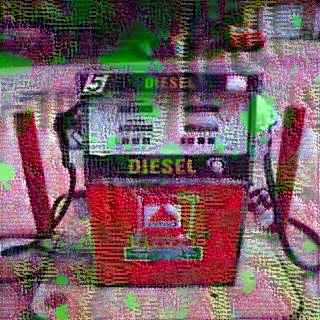}
        \includegraphics[width=.98\linewidth]{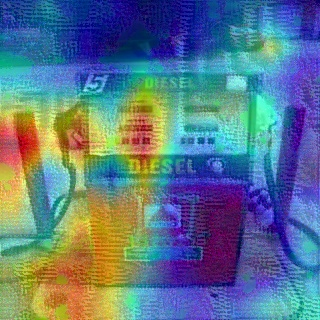}
        \includegraphics[width=.98\linewidth]{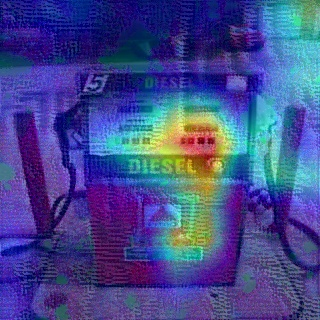}
        \caption{$\epsilon = 0.3$}
    \end{subfigure}
    % parachute
    \centering
    \begin{subfigure}{.075\linewidth}
        \centering
        \includegraphics[width=.98\linewidth]{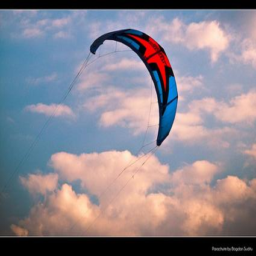}
        \includegraphics[width=.98\linewidth]{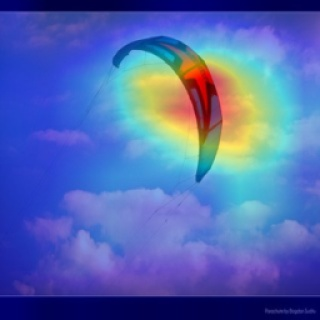}
        \includegraphics[width=.98\linewidth]{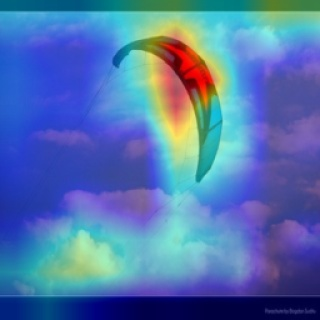}
        \caption{$\epsilon = 0$}
    \end{subfigure}
    \begin{subfigure}{.075\linewidth}
        \centering
        \includegraphics[width=.98\linewidth]{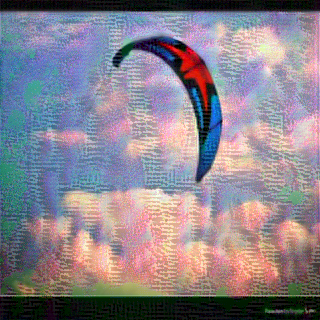}
        \includegraphics[width=.98\linewidth]{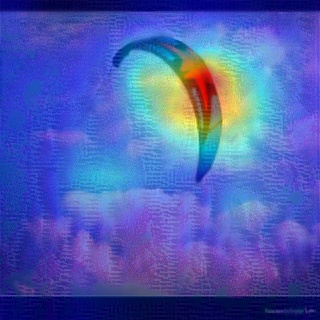}
        \includegraphics[width=.98\linewidth]{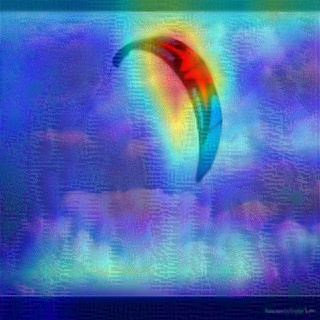}
        \caption{$\epsilon = 0.1$}
    \end{subfigure}
    \begin{subfigure}{.075\linewidth}
        \centering
        \includegraphics[width=.98\linewidth]{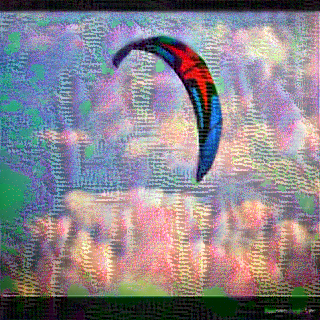}
        \includegraphics[width=.98\linewidth]{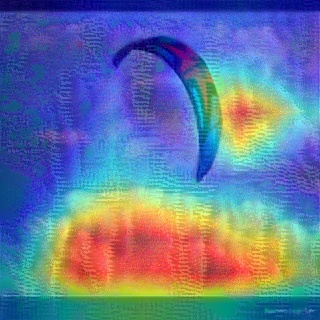}
        \includegraphics[width=.98\linewidth]{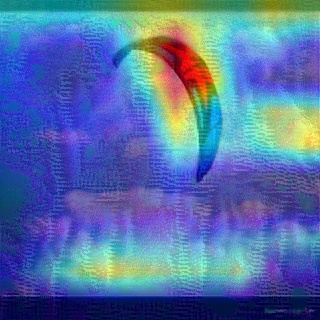}
        \caption{$\epsilon = 0.2$}
    \end{subfigure}
    \begin{subfigure}{.075\linewidth}
        \centering
        \includegraphics[width=.98\linewidth]{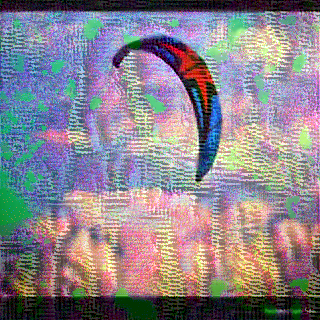}
        \includegraphics[width=.98\linewidth]{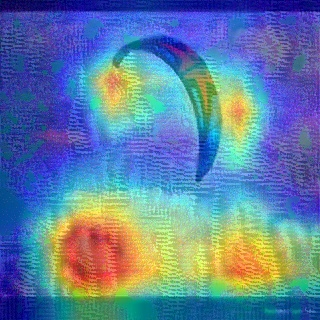}
        \includegraphics[width=.98\linewidth]{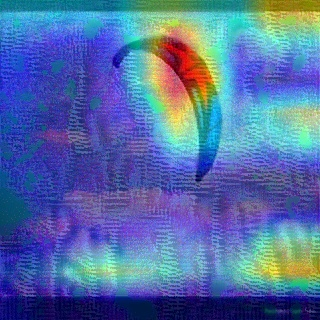}
        \caption{$\epsilon = 0.3$}
    \end{subfigure}
    % chain saw
    \centering
    \begin{subfigure}{.075\linewidth}
        \centering
        \includegraphics[width=.98\linewidth]{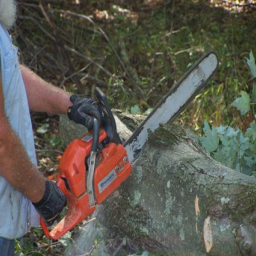}
        \includegraphics[width=.98\linewidth]{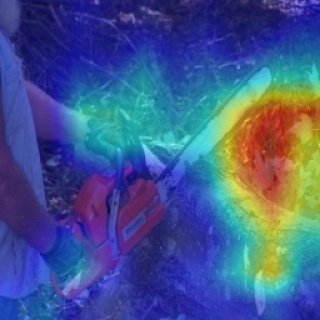}
        \includegraphics[width=.98\linewidth]{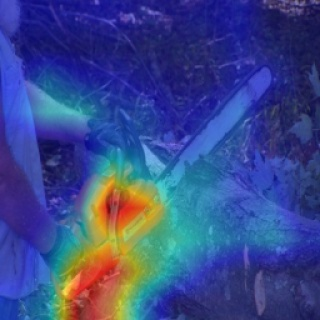}
        \caption{$\epsilon = 0$}
    \end{subfigure}
    \begin{subfigure}{.075\linewidth}
        \centering
        \includegraphics[width=.98\linewidth]{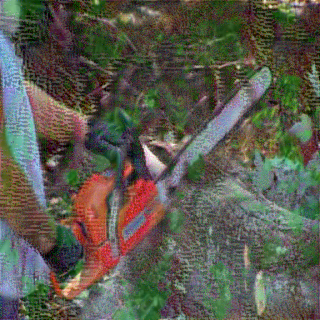}
        \includegraphics[width=.98\linewidth]{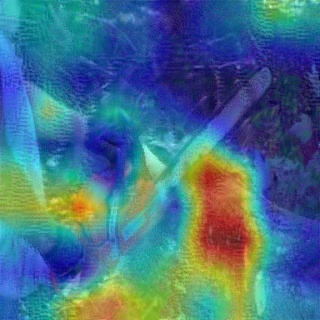}
        \includegraphics[width=.98\linewidth]{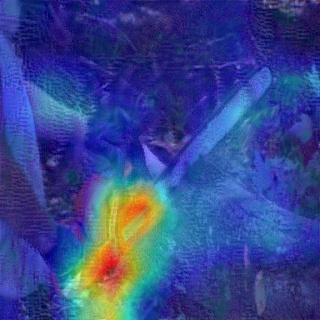}
        \caption{$\epsilon = 0.1$}
    \end{subfigure}
    \begin{subfigure}{.075\linewidth}
        \centering
        \includegraphics[width=.98\linewidth]{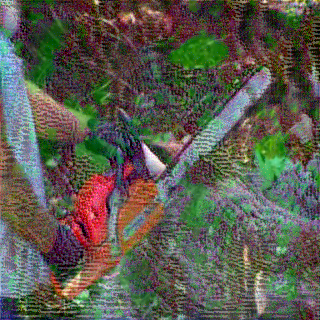}
        \includegraphics[width=.98\linewidth]{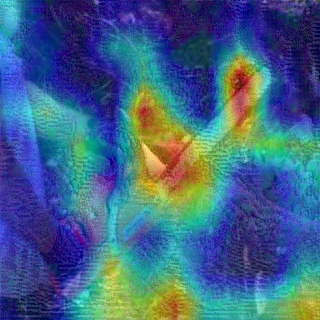}
        \includegraphics[width=.98\linewidth]{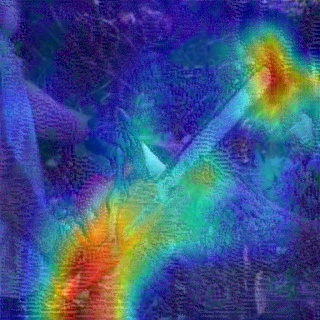}
        \caption{$\epsilon = 0.2$}
    \end{subfigure}
    \begin{subfigure}{.075\linewidth}
        \centering
        \includegraphics[width=.98\linewidth]{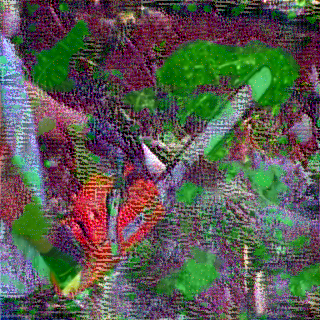}
        \includegraphics[width=.98\linewidth]{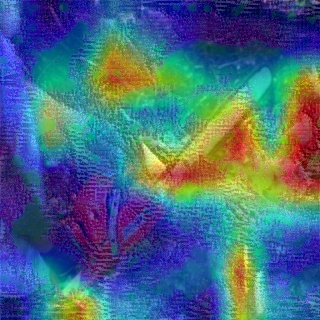}
        \includegraphics[width=.98\linewidth]{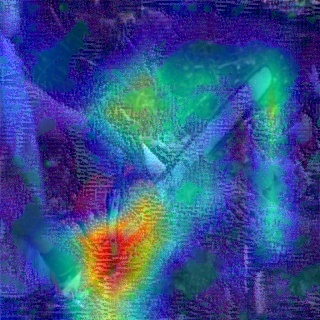}
        \caption{$\epsilon = 0.3$}
    \end{subfigure}
    % church
    \centering
    \begin{subfigure}{.075\linewidth}
        \centering
        \includegraphics[width=.98\linewidth]{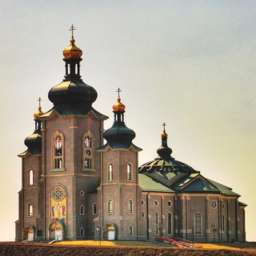}
        \includegraphics[width=.98\linewidth]{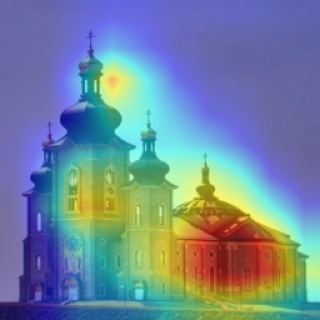}
        \includegraphics[width=.98\linewidth]{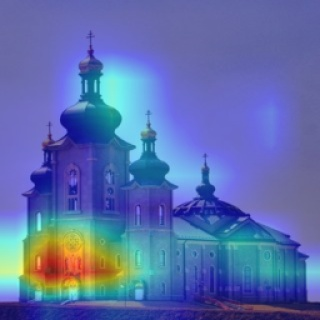}
        \caption{$\epsilon = 0$}
    \end{subfigure}
    \begin{subfigure}{.075\linewidth}
        \centering
        \includegraphics[width=.98\linewidth]{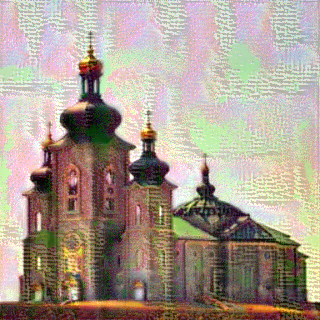}
        \includegraphics[width=.98\linewidth]{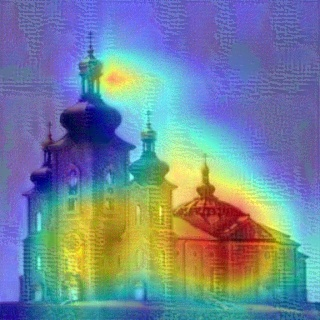}
        \includegraphics[width=.98\linewidth]{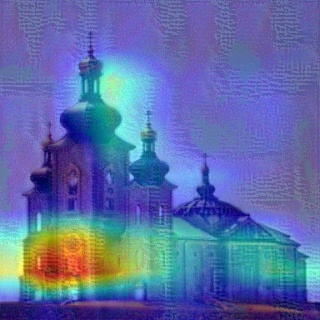}
        \caption{$\epsilon = 0.1$}
    \end{subfigure}
    \begin{subfigure}{.075\linewidth}
        \centering
        \includegraphics[width=.98\linewidth]{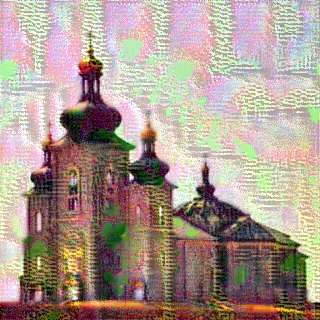}
        \includegraphics[width=.98\linewidth]{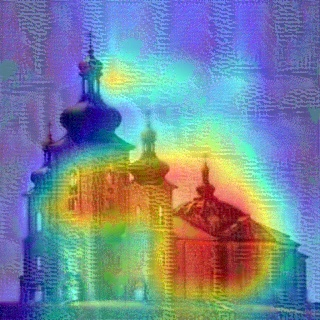}
        \includegraphics[width=.98\linewidth]{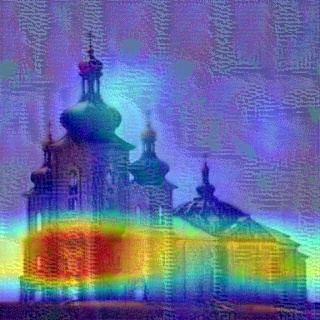}
        \caption{$\epsilon = 0.2$}
    \end{subfigure}
    \begin{subfigure}{.075\linewidth}
        \centering
        \includegraphics[width=.98\linewidth]{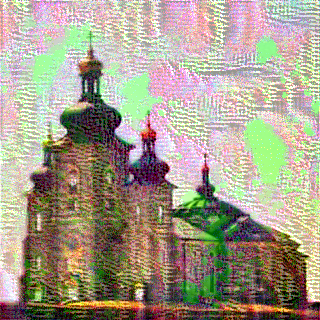}
        \includegraphics[width=.98\linewidth]{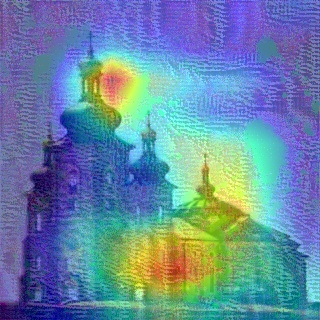}
        \includegraphics[width=.98\linewidth]{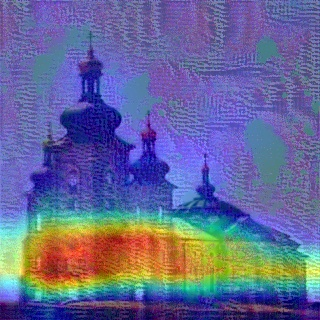}
        \caption{$\epsilon = 0.3$}
    \end{subfigure}
    \caption{Grad-Cam visualization of VGG11 based transfer attacks. Top, middle and bottom of each column presents the (adversarial) image, visualization of ResNet18 and that of SF-ResNet18.}
    \label{apxfig:grad_cam}
\end{figure*}   

\begin{figure*}[t]
    \centering
    \begin{subfigure}{.075\linewidth}
        \centering
        \includegraphics[width=.98\linewidth]{figure/apx/golf.jpg}
        \includegraphics[width=.98\linewidth]{figure/apx/cam_rgbgolf_00.jpg}
        \includegraphics[width=.98\linewidth]{figure/apx/cam_fgolf_00.jpg}
        \caption{$\epsilon = 0$}
    \end{subfigure}
    \begin{subfigure}{.075\linewidth}
        \centering
        \includegraphics[width=.98\linewidth]{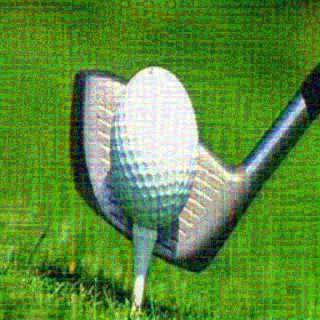}
        \includegraphics[width=.98\linewidth]{figure/apx/fcam_rgbgolf_01.jpg}
        \includegraphics[width=.98\linewidth]{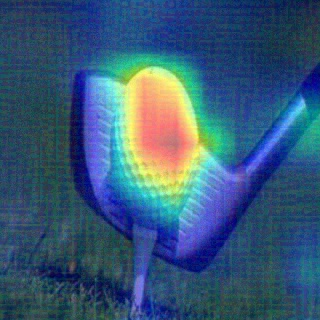}
        \caption{$\epsilon = 0.1$}
    \end{subfigure}
    \begin{subfigure}{.075\linewidth}
        \centering
        \includegraphics[width=.98\linewidth]{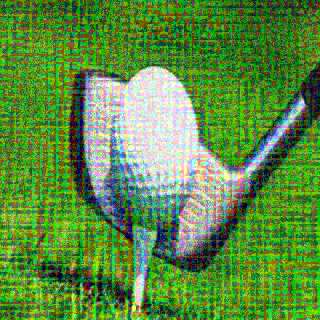}
        \includegraphics[width=.98\linewidth]{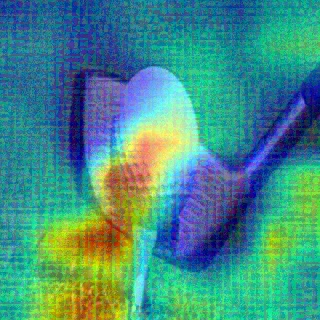}
        \includegraphics[width=.98\linewidth]{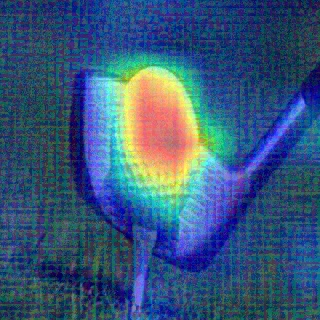}
        \caption{$\epsilon = 0.2$}
    \end{subfigure}
    \begin{subfigure}{.075\linewidth}
        \centering
        \includegraphics[width=.98\linewidth]{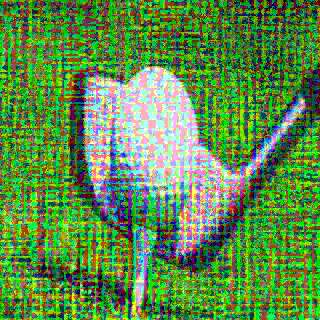}
        \includegraphics[width=.98\linewidth]{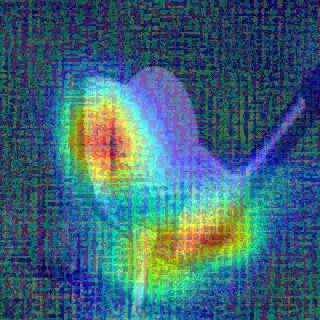}
        \includegraphics[width=.98\linewidth]{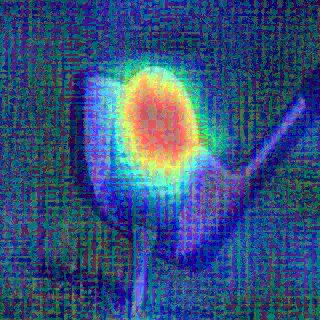}
        \caption{$\epsilon = 0.3$}
    \end{subfigure}
    %gas pump
    \centering
    \begin{subfigure}{.075\linewidth}
        \centering
        \includegraphics[width=.98\linewidth]{figure/apx/gas.jpg}
        \includegraphics[width=.98\linewidth]{figure/apx/cam_rgbgas_00.jpg}
        \includegraphics[width=.98\linewidth]{figure/apx/cam_fgas_00.jpg}
        \caption{$\epsilon = 0$}
    \end{subfigure}
    \begin{subfigure}{.075\linewidth}
        \centering
        \includegraphics[width=.98\linewidth]{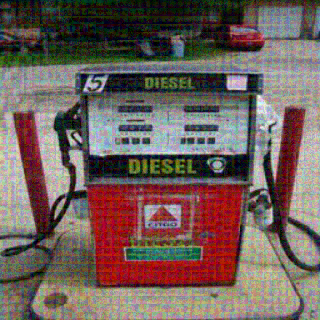}
        \includegraphics[width=.98\linewidth]{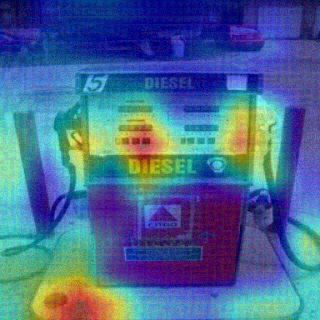}
        \includegraphics[width=.98\linewidth]{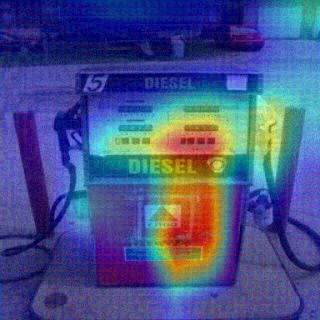}
        \caption{$\epsilon = 0.1$}
    \end{subfigure}
    \begin{subfigure}{.075\linewidth}
        \centering
        \includegraphics[width=.98\linewidth]{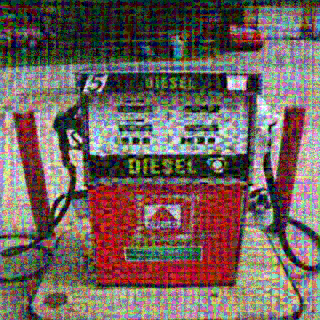}
        \includegraphics[width=.98\linewidth]{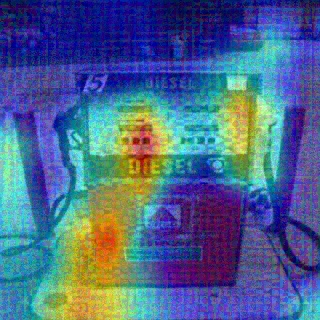}
        \includegraphics[width=.98\linewidth]{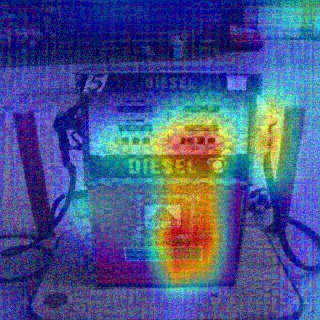}
        \caption{$\epsilon = 0.2$}
    \end{subfigure}
    \begin{subfigure}{.075\linewidth}
        \centering
        \includegraphics[width=.98\linewidth]{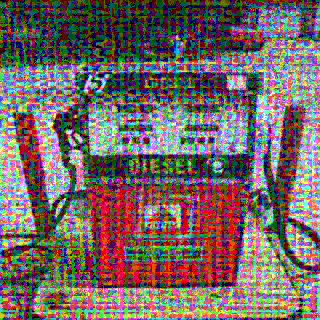}
        \includegraphics[width=.98\linewidth]{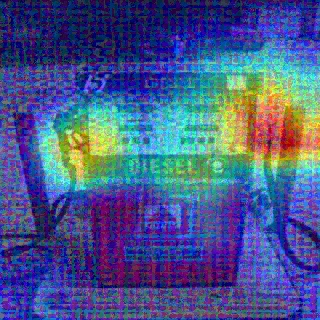}
        \includegraphics[width=.98\linewidth]{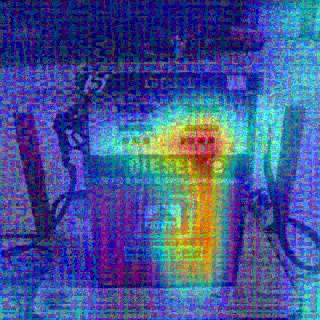}
        \caption{$\epsilon = 0.3$}
    \end{subfigure}
    % parachute
    \centering
    \begin{subfigure}{.075\linewidth}
        \centering
        \includegraphics[width=.98\linewidth]{figure/apx/chute.jpg}
        \includegraphics[width=.98\linewidth]{figure/apx/cam_rgbchute_00.jpg}
        \includegraphics[width=.98\linewidth]{figure/apx/cam_fchute_00.jpg}
        \caption{$\epsilon = 0$}
    \end{subfigure}
    \begin{subfigure}{.075\linewidth}
        \centering
        \includegraphics[width=.98\linewidth]{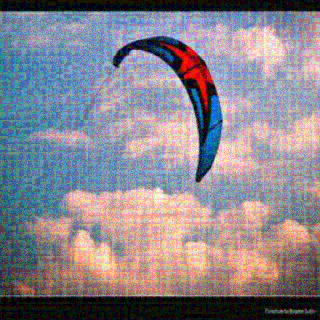}
        \includegraphics[width=.98\linewidth]{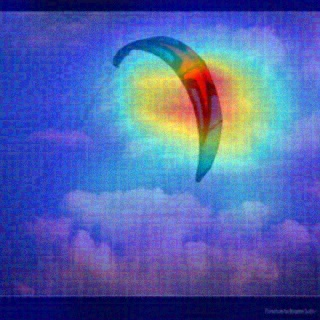}
        \includegraphics[width=.98\linewidth]{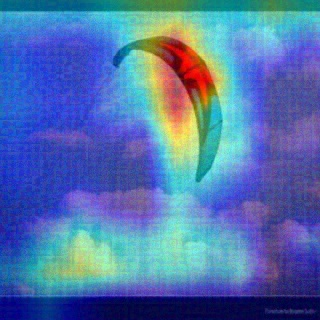}
        \caption{$\epsilon = 0.1$}
    \end{subfigure}
    \begin{subfigure}{.075\linewidth}
        \centering
        \includegraphics[width=.98\linewidth]{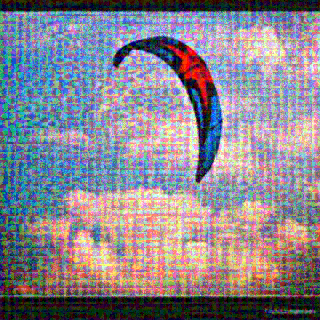}
        \includegraphics[width=.98\linewidth]{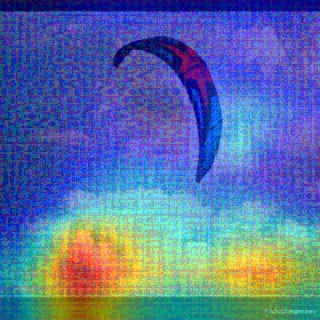}
        \includegraphics[width=.98\linewidth]{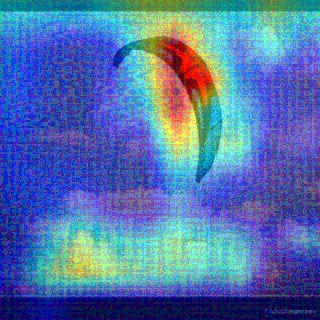}
        \caption{$\epsilon = 0.2$}
    \end{subfigure}
    \begin{subfigure}{.075\linewidth}
        \centering
        \includegraphics[width=.98\linewidth]{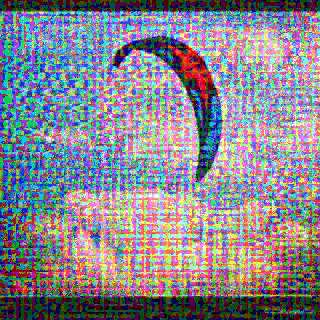}
        \includegraphics[width=.98\linewidth]{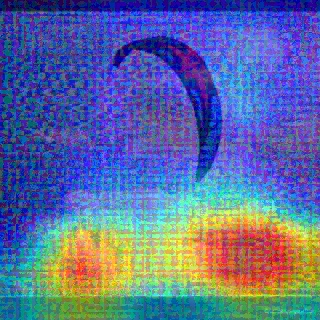}
        \includegraphics[width=.98\linewidth]{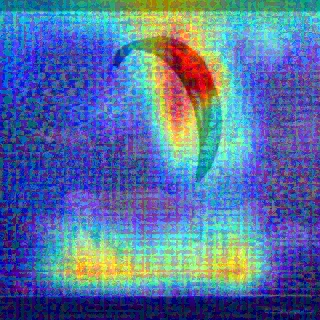}
        \caption{$\epsilon = 0.3$}
    \end{subfigure}
    \caption{Grad-Cam visualization of SF-VGG11 based transfer attacks. Top, middle and bottom of each column presents the (adversarial) image, visualization of ResNet18 and that of SF-ResNet18.}
    \label{apxfig:grad_cam_sf}
\end{figure*}
